# Supplementary material for: Accelerating all-atom simulations and gaining mechanistic understanding of biophysical systems through State Predictive Information Bottleneck
Source: arXiv:2112.11201 ancillary file (2021-12-21)
Supplement: Supplementary file 1 [file Shams_SI.pdf]

# Supplementary Material: Accelerating all-atom simulations and gaining mechanistic understanding of biophysical systems through State Predictive Information Bottleneck

**Mehdi, Wang, Pant and Tiwary**

## I. MOLECULAR DYNAMICS (MD) PARAMETERS

CHARMM-GUI[1] web server was used to generate both $(Aib)_9$ and BA-DMPC systems with solvation boxes of sizes 3.5nm x 3.5nm x 3.5nm and 5.0nm x 5.0nm x 9.0nm respectively. All well-tempered metadynamics simulations were performed using biasfactor 10.0, gaussian initial height 10.0 kJ/mol, pace 2.0 ps, and 20% of standard deviation of SPIB RCs from previous round of simulation as sigmas for both systems.

## II. MD DETAILS AND EXTENDED TRAJECTORIES

### A. Chiral transitions in $(Aib)_9$

The $500ns$ unbiased MD was extended to $3.8\mu s$ which served as the unbiased benchmark simulation. The $\zeta$ OP time series indicates only two complete back and forth between L and R metastable states as shown in Supplementary Fig. 1(a).

The $500ns$ unbiased MD was then used to train SPIB models with a 2-dimensional RC based on temporal and structural initial state assignment schemes respectively. For temporal scheme, 10 initial states were assigned to the $500ns$ trajectory by sequentially dividing it into 10 equal slices of $50ns$ each. Based on this 2-d RC using time delay, $\Delta t = 2ns$, a $485ns$ long metadynamics was performed. $\zeta$ time series for this trajectory is shown in Supplementary Fig. 1(b) which clearly indicates enhanced sampling. Time length of each of the slices of temporal scheme should be short enough so that different key metastable states do not get mixed with each other under same initial states.

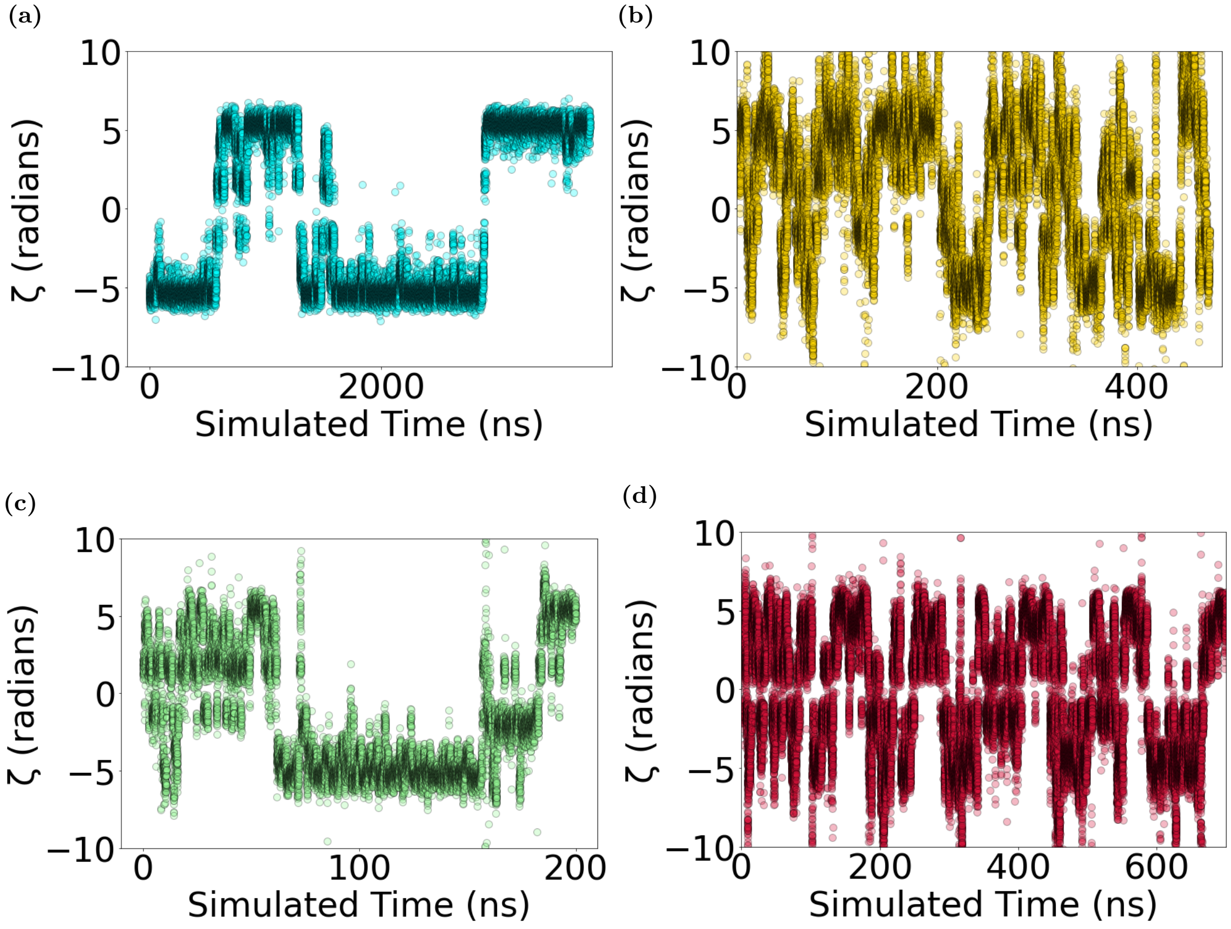


**Supplementary Figure 1:** $\zeta$ time series for (a) $3.8\mu$s unbiased, (b) $485ns$ biased MD based on temporal initial state assignment, (c) $200ns$ biased MD based on structural state assignment, (d) $700ns$ second round of biased MD based on the first round of structural state assignment as shown in (c).

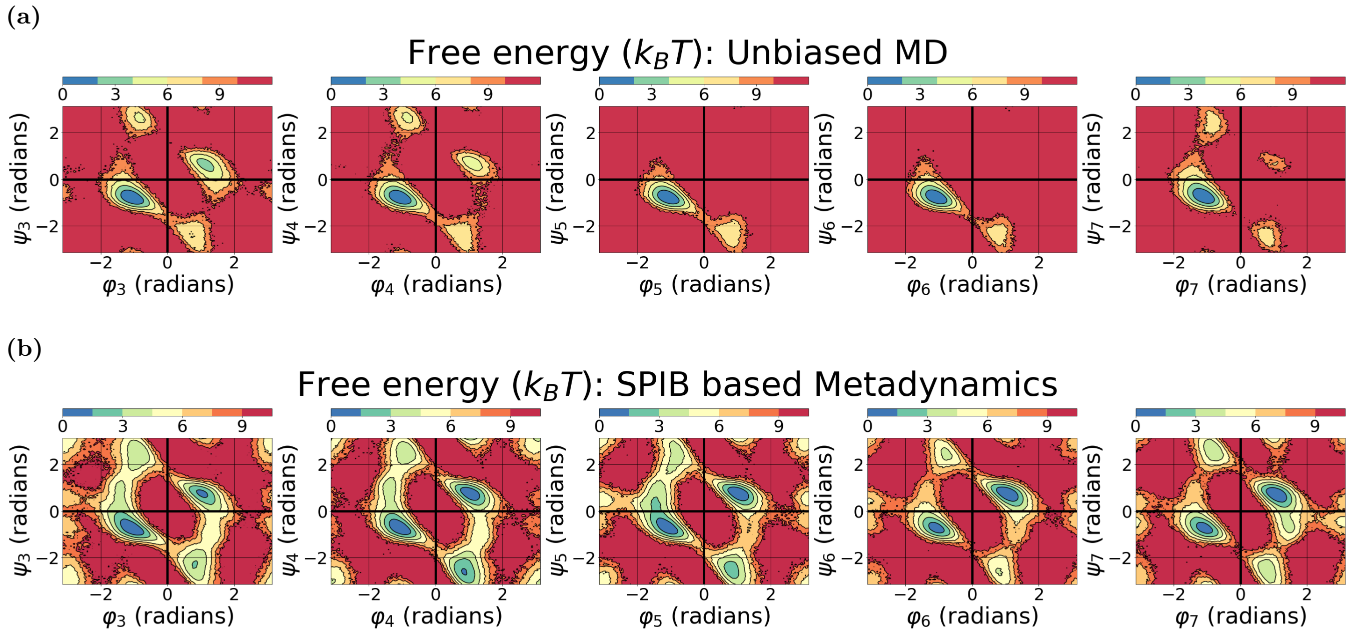


**Supplementary Figure 2:** Free energy along $(\phi, \psi)$ space for (a) $500ns$ Unbiased MD that was used to train SPIB models, (b) $700ns$ SPIB augmented metadynamics demonstrating improved sampling.

The structural scheme was implemented by considering the $\phi$ dihedral angles of the inner 5 residues. If $\phi \geq 0$ for a particular residue, it was assigned label '1' and '0' if $\phi < 0$. For example, when the inner 5 residues assume values $\phi = -0.6, 0.3, 0.8, -0.9, 1.1$ radians respectively, we assigned a unique initial label '01101' or equivalently state '18' in SPIB to that timestep. Based on this structural scheme and time delat, $\Delta t = 1ns$, a $200ns$ long metadynamics was performed as shown in Supplementary Fig. 1(c). Subsequently, this trajectory was used as the input to train a second round of SPIB model using time delay, $\Delta t = 0.75ns$ based on which a $700ns$ metadynamics simulation was performed (Supplementary Fig. 1(d)). A comparison between Supplementary Fig. 1(c), and Supplementary Fig. 1(d) clearly indicates that the second round of SPIB generated an improved RC. This improvement was due to the fact that more metastable states including both state L and state R were present in the input trajectory for round 2 training.

### B. BA permeation through phospholipid bilayer

We began our study on BA-DMPC by conducting a $500ns$ long unbiased MD simulation of the BA-DMPC system, starting from the configuration where BA was outside the membrane along the +Z direction (Fig. 4(a)). It is evident from $d1_Z$ that once BA enters the membrane, it remains trapped close to the surface region of the membrane and a complete permeation event was not observed during this unbiased MD.

Two independent 25 ns simulations for BA-DMPC were conducted where BA was initially placed outside the membrane along +Z and -Z directions respectively. Subsequently, initial states were assigned to this combined 50 ns dataset from the *a priori* infomration that the phospholipid bilayer has been modelled along X-Y axes of the simulation box and BA needs to cross the membrane along Z direction. Additionally, there is a possibility that the angle between BA and Z axis may contain permeation insights due to BA having polar (=O, -OH) groups. Hence, for this system it is reasonable to consider $d1_Z, \theta_Z$ for assigning the initial states. Regular space clustering scheme of PyEMMA (dmin = 1.0) [2] python library was employed to obtain 22 initial states as shown in Supplementary Fig. 3(b,c). Afterwards, 1-d RC was learnt with 8 converged SPIB states using time delay, $\Delta t = 2ps.$ as shown in Supplementary Fig. 3(d). Projection of this RC along $(d1_Z, \theta Z)$ clearly shows that SPIB was able to capture the key metastable states of this system (Supplementary Fig. 3(e)). Finally, a $500ns$ long metadynamics was performed based on this 1-d RC at 298.15K and 1 atm. During this simulation, the average phosphate center-of-mass of the upper and lower membrane leaflets are located at 1.85 and -1.84 nm from the membrane COM respectively.

To analyze this trajectory using SPIB, initial states were assigned by discretizing $d1_Z$ into 8 different state labels as shown in Supplementary Fig. 4(a). Since, round 1 of SPIB demonstrated minimal dependence of the converged states on $\theta_Z$ (Supplementary Fig. 3(e)), only $d1_Z$ was used for assigning initial states for round 2. Subsequently a 1-d RC was learnt by using time delay, $\Delta t = 20ps$ as shown in Supplementary Fig. 4(b). Although $\theta_Z$ was not useful in

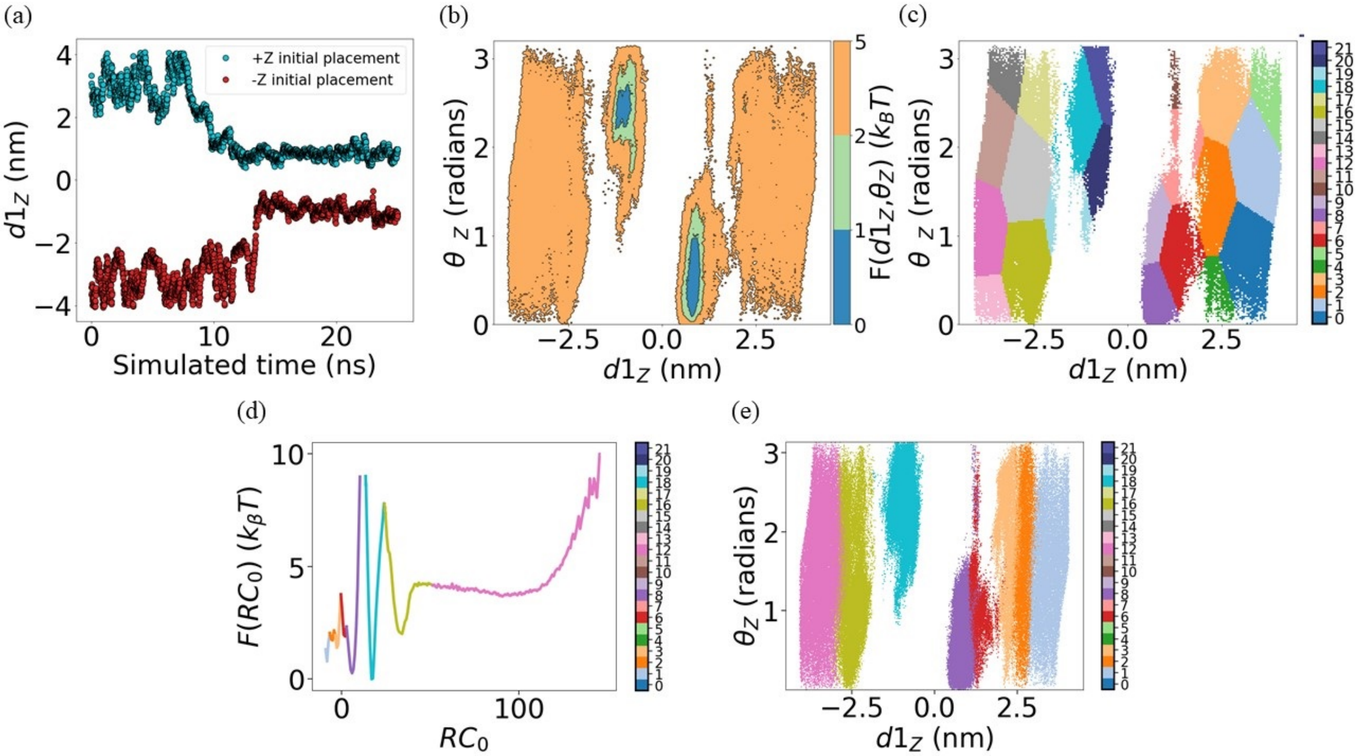


**Supplementary Figure 3:** (a) Two independent trajectories with BA initially placed outside the membrane along +Z and -Z directions respectively, (b) free energy along $(d1_Z, \theta_Z)$ from combined trajectory dataset, (c) 22 initial state assignments using regular space clustering algorithm of PyEMMA, (d) 1-d SPIB RC using time delay, $\Delta t = 2ps$ highlights different converged states corresponding to $F(RC_0)$ minima regions, (e) converged state labels projected on $(d1_Z, \theta_Z)$ space.

differentiating the metastable states in round 1, for round 2 it was important in identifying the key permeation barrier (Fig. 4(c)). This was because the combined $50ns$ unbiased trajectory did not contain any data corresponding to BA crossing the membrane center. It should be noted that, round 2 of SPIB performed on metadynamics trajectory data captured the importance of $\theta_Z$ even though the initial state assignment was performed by only considering $d1_Z$ for this round. This highlights the robustness and a key strength of SPIB.

## III. NEURAL NETWORK STRUCTURE AND SPIB HYPERPARAMETES

SPIB neural network is constructed from nonlinear encoder and decoder with two hidden layers each. The SPIB hyperparameters for these two systems are provided in Supplementary Table 1.

| System | Initial labelling scheme | RC dimensionality | Time delay | Beta | Learning rate |
|---|---|---|---|---|---|
| $(Aib)_9$ | temporal | 2-d | 2 ns | 0.001 | 0.0001 |
| $(Aib)_9$ | structural | 2-d | 1 ns | 0.0005 | 0.0001 |
| $(Aib)_9$ | structural, round 2 | 2-d | 0.75 ns | 0.01 | 0.0001 |
| $(Aib)_9$ | structural, round 3 | 2-d | 0.3 ns | 0.01 | 0.0001 |
| BA-DMPC | $(d1_Z,\theta_Z)$ | 1-d | 2 ps | 0.001 | 0.000005 |
| BA-DMPC | $(d1_Z,\theta_Z)$, round 2 | 1-d | 20 ps | 0.0001 | 0.000001 |

**Supplementary Table 1: SPIB hyperparameters**

An important hyperparameter of SPIB that one can adjust manually is the time-delay $\Delta t$. This parameter denotes how far into the future we are training the model to make predictions and correspondingly, how coarse-grained the predicted metastable states are, with the predicted number of states expected to decrease monotonically as a function of time as shown in Supplementary Fig. 5(b)). All ANN models were trained until SPIB outputs converged. The convergence can be quantified by monitoring the number and population of different states, which should both no

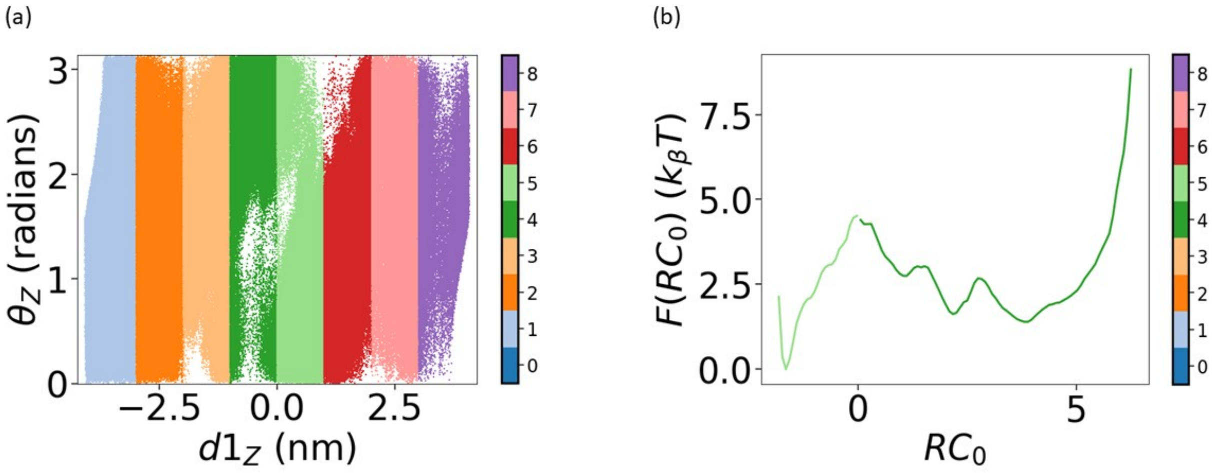


**Supplementary Figure 4:** (a) Initial state assignments for analyzing the 500$ns$ BA-DMPC metadynamics trajectory, (b) 1-d RC using time delay, $\Delta t = 20ps$ highlights two converged states.

longer change as a function of further iterations as shown in Supplementary Fig. 5 (a). In this work, we employed an updated version of SPIB (ver_July2021), with an improved implementation of the state convergence criterion.

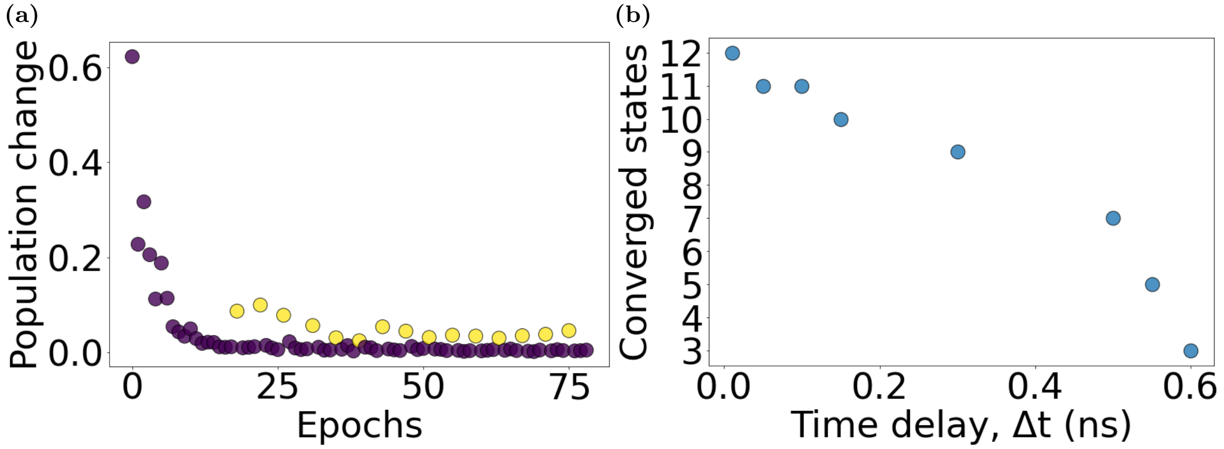


**Supplementary Figure 5:** (a) SPIB state population change measure vs. iterations/epochs for an example ANN model training process for the $(Aib)_9$ system. Yellow color indicates a label update. No significant state population change is observed after convergence, (b) number of converged states detected by SPIB for the $(Aib)_9$ system decreased monotonically with time.

**References**

[1] J. Lee, X. Cheng, J. M. Swails, M. S. Yeom, P. K. Eastman, J. A. Lemkul, S. Wei, J. Buckner, J. C. Jeong, Y. Qi, et al., Journal of chemical theory and computation **12**, 405 (2016).

[2] M. K. Scherer, B. Trendelkamp-Schroer, F. Paul, G. Pérez-Hernández, M. Hoffmann, N. Plattner, C. Wehmeyer, J.-H. Prinz, and F. Noé, Journal of chemical theory and computation **11**, 5525 (2015).
